# Supplementary material for: Size effects on supercooling phenomena in strongly correlated electron systems: IrTe$_2$ and $\theta$-(BEDT-TTF)$_2$RbZn(SCN)$_4$
Source: arXiv:1802.09739 source file (2018-02-27)
Supplement: Supplementary file 1 [file Oike_sizeeffect_supple.pdf]

Supplementary Material for

# Size effects on supercooling phenomena in strongly correlated electron systems: $IrTe_2$ and $\theta$-$(BEDT\text{-}TTF)_2RbZn(SCN)_4$

H. Oike,[1,*] M. Suda,[2] M. Kamitani,[1] A. Ueda,[3] H. Mori,[3] Y. Tokura,[1,4] H. M. Yamamoto,[2] and F. Kagawa[1,4,†]

[1] *RIKEN Center for Emergent Matter Science (CEMS), Wako 351-0198, Japan*

[2] *Research Center for Integrative Molecular System (CIMoS), Institute for Molecular Science, Okazaki 444-8585, Japan*

[3] *The Institute for Solid State Physics, The University of Tokyo, Kashiwa 277-8581, Japan*

[4] *Department of Applied Physics, The University of Tokyo, Tokyo 113-8656, Japan*

*E-mail: hiroshi.oike@riken.jp

†E-mail: fumitaka.kagawa@riken.jp

## Sample preparation

### $IrTe_2$

Bulk IrTe crystals were synthesized using the Te-flux method according to the literature [S1]. To study the transition behavior in samples much smaller than the bulk crystals, submicrometer-thick crystals were exfoliated from a bulk single crystal with Scotch tape and transferred onto silicon or sapphire substrates. The electrodes were prepared on the sample surface and substrate using photolithography methods, and they were connected by tungsten deposition using a focused-ion beam (FIB). An image of the typical sample is shown in Fig. S14(a). The sample thickness was measured by using scanning electron microscopy (SEM).

### θ-$(BEDT\text{-}TTF)_2RbZn(SCN)_4$

Single crystals of θ-$(BEDT\text{-}TTF)_2RbZn(SCN)_4$ were synthesized via the galvanostatic anodic oxidation of BEDT-TTF in an Ar atmosphere, using the electrolyte as RbSCN and $Zn(SCN)_2$ in 1,1,2-trichloroethane (20% methanol). After we applied a current of approximately 1 μA for 12–24 h, single crystals with various sizes were obtained. To minimize the strain effects from the substrates, small single crystals with four gold wires (15 μm-ϕ) were placed on a Teflon sheet with no glue, such that the samples could be considered as nominally free-standing except for the possible strains that from the gold wires. An image of the typical microcrystals is shown in Fig. S14(b).

## Supplementary references

[S1] M. J. Eom, K. Kim, Y. J. Jo, J. J. Yang, E. S. Choi, B. I. Min, J.-H. Park, S.-W. Cheong, and J. S. Kim, Phys. Rev. Lett. **113**, 266406 (2014).

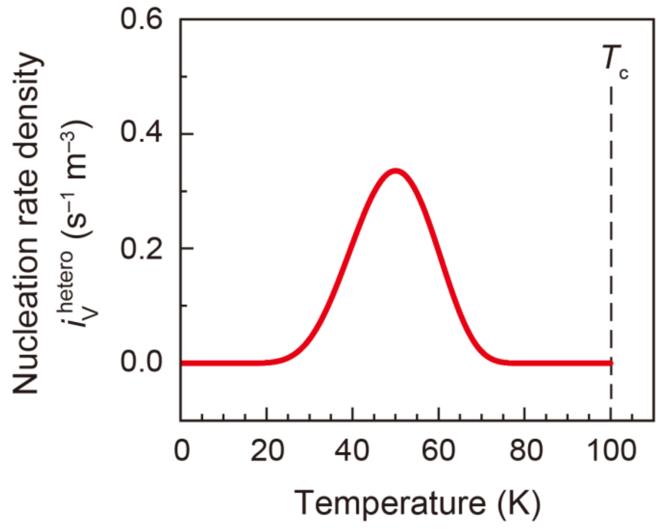


Fig. S1: Linear-scale representation of the modeled temperature dependence of the nucleation rate density $I_V(T)$ for the simulation. The logarithmic-scale representation is shown in the main text (Fig. 2).

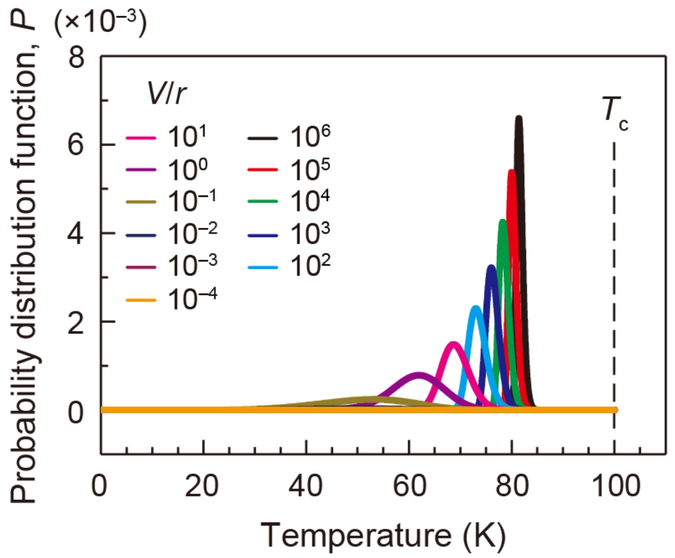


Fig. S2: Linear-scale representation of the calculated probability distribution function $P(T)$ regarding the occurrence of the first nucleation event. The logarithmic-scale representation is shown in the main text [Fig. 3(a)].

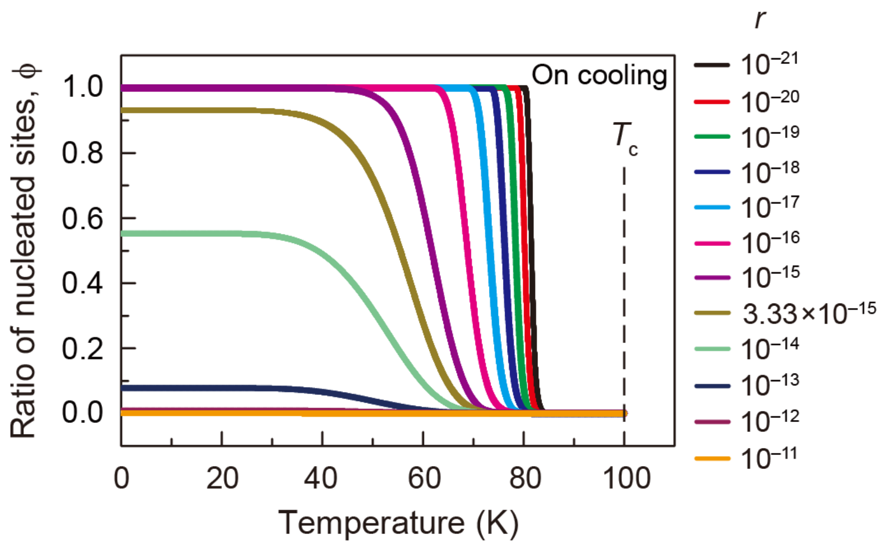


Fig. S3: Temperature dependence of the calculated ratio of nucleation-completed sites to the total potential nucleation sites for the case of zero growth speed. For the calculation, $\rho_{\mathrm{defect}}$ ($\equiv i_{\mathrm{v}}^{\mathrm{hetero}}(T)/I_{\mathrm{defect}}(T)$) = $10^{15}$ is used.

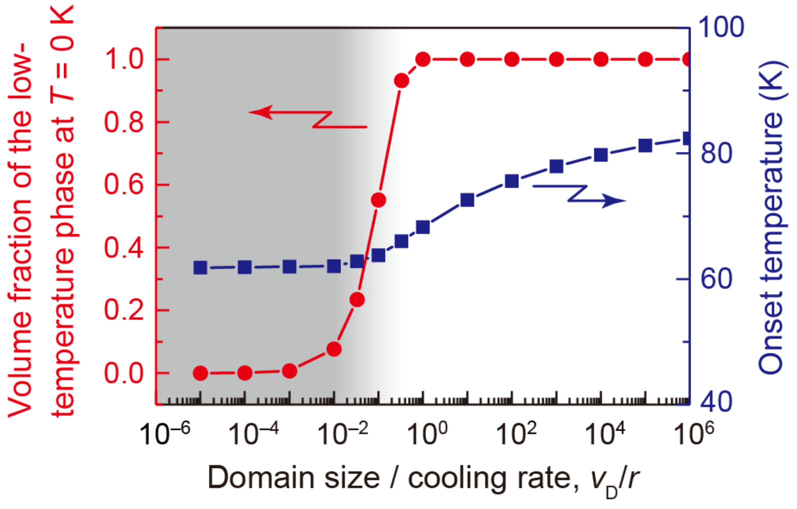


Fig. S4: Simulated cooling-rate dependence of the volume fraction of the low-temperature phase at $T$ = 0 K (left axis) and the onset temperature of the transition (right axis), which were extracted from the transition behavior in the main text, Fig. 4. The unit of $v_D/r$ is [$K^{-1}$ s $m^3$].

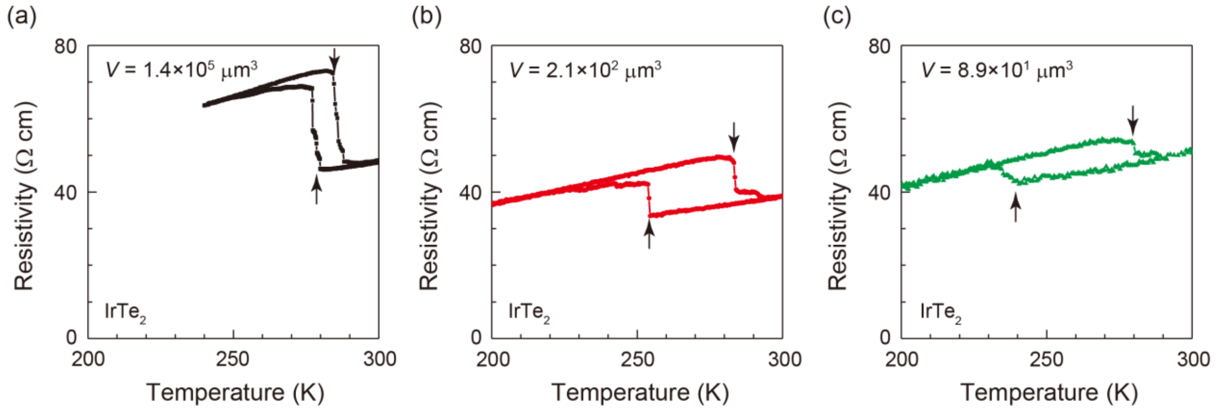


Fig. S5: Temperature-resistivity profiles of $IrTe_2$ with different sample volumes: (a) $1.4\times10^5$ $\mu m^3$, (b) $2.1\times10^2$ $\mu m^3$, and (c) $8.9\times10^1$ $\mu m^3$. The transition-onset temperatures are indicated by arrows.

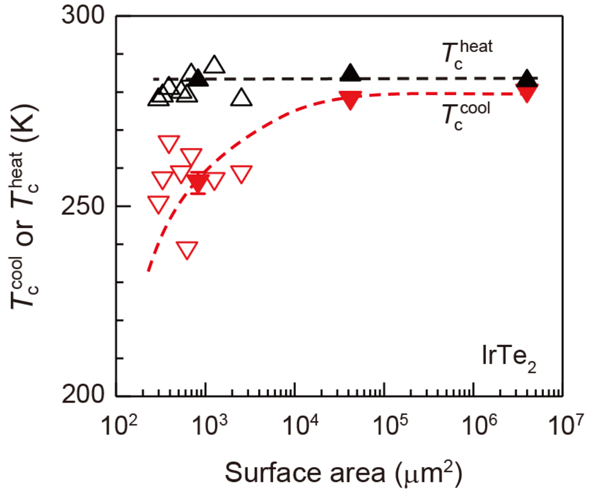


Fig. S6: $T_c^{cool}$ and $T_c^{heat}$ variations with the sample surface area in $IrTe_2$. The red and black symbols represent $T_c^{cool}$ and $T_c^{heat}$, respectively. For selected samples (closed symbols), we examined the reproducibility of the transition temperature by repeating certain experiments; the observed variations in $T_c^{cool}$ or $T_c^{heat}$ are represented by error bars. The broken lines are drawn as a guide for the eyes.

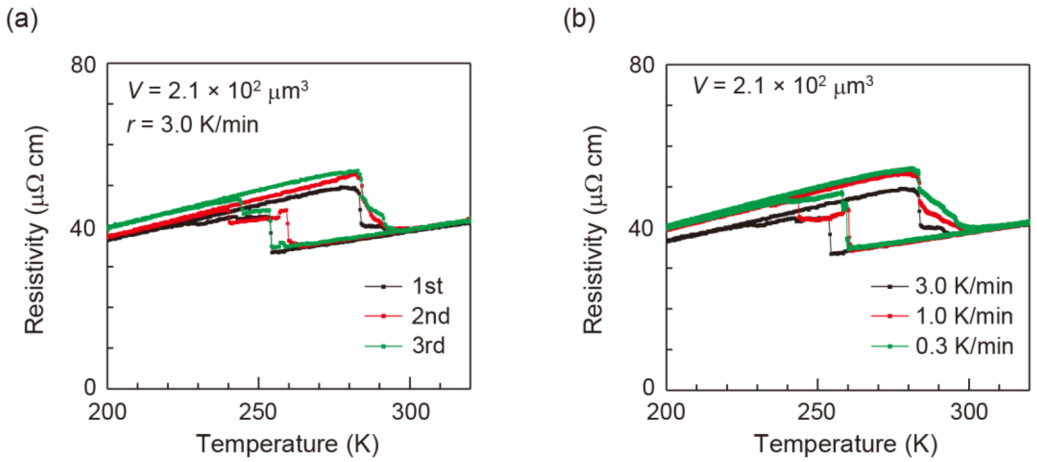


Fig. S7: Temperature-resistivity profile in $IrTe_2$ with a volume of $2.1\times10^2$ μm$^3$: (a) Reproducibility and (b) cooling-rate dependence. In the repeated thermal-cycling experiments, the transition temperature upon cooling $T_c^{cool}$ exhibits variations, which are represented by error bars in Fig. 5 in the main text. The cooling-rate dependence of $T_c^{cool}$ in this range is comparable to the variations with thermal cycling.

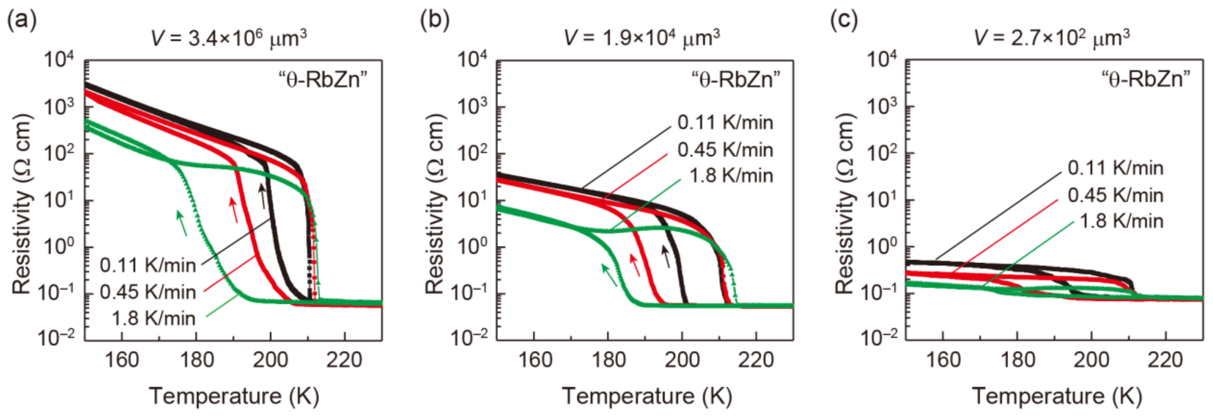


Fig. S8: Temperature-resistivity profiles of θ-(BEDT-TTF)$_2$RbZn(SCN)$_4$ with different temperature-sweep rates and sample volumes: (a) $3.4 \times 10^6$ μm$^3$; (b) $1.9 \times 10^4$ μm$^3$; and (c) 2.7 × $10^2$ μm$^3$.

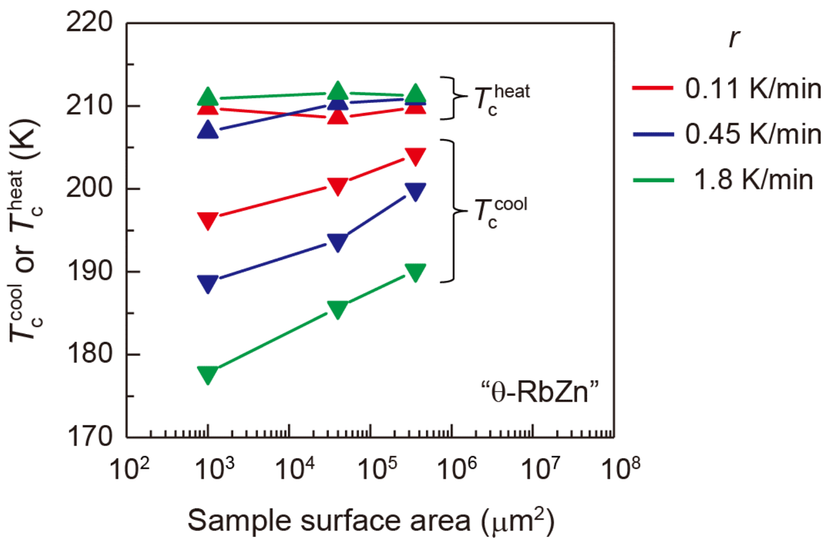


Fig. S9: $T_c^{cool}$ and $T_c^{heat}$ variations with the sample surface area in θ-(BEDT-TTF)$_2$RbZn(SCN)$_4$.

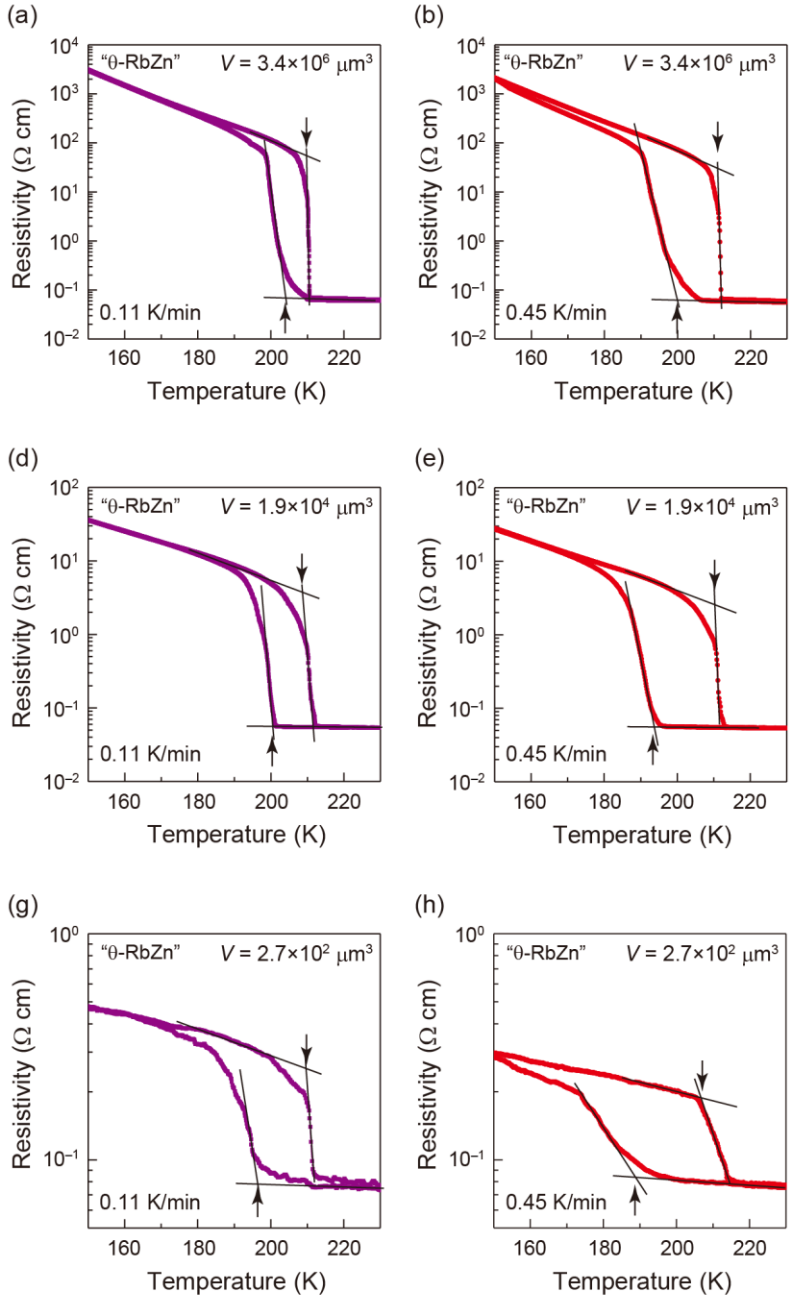


Fig. S10: Temperature-resistivity profiles of θ-(BEDT-TTF)$_2$RbZn(SCN)$_4$ with different temperature-sweep rates and sample volumes: (a–c) $3.4\times10^6$ μm$^3$, (d–f) $1.9\times10^4$ μm$^3$, and (g–i) $2.7\times10^2$ μm$^3$. The transition-onset temperatures are indicated by arrows.

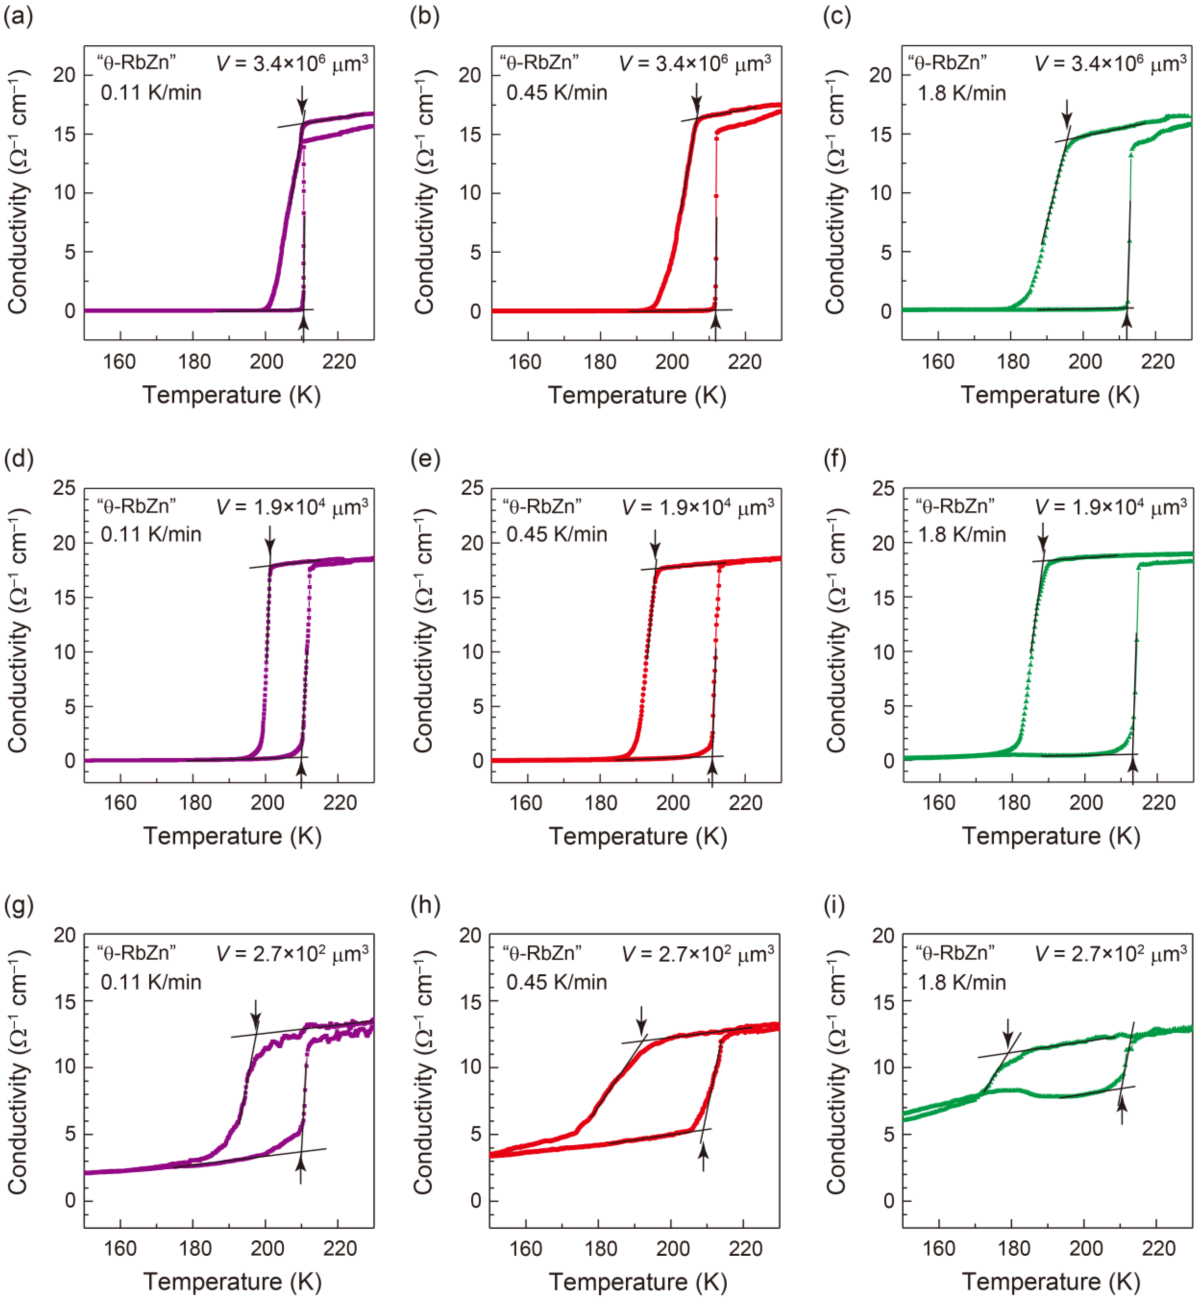


Fig. S11: Temperature-conductivity profiles of θ-(BEDT-TTF)$_2$RbZn(SCN)$_4$ with different temperature-sweep rates and sample volumes: (a–c) 3.4×10$^6$ μm$^3$, (d–f) 1.9×10$^4$ μm$^3$, and (g–i) 2.7×10$^2$ μm$^3$. The transition-onset temperatures are indicated by arrows.

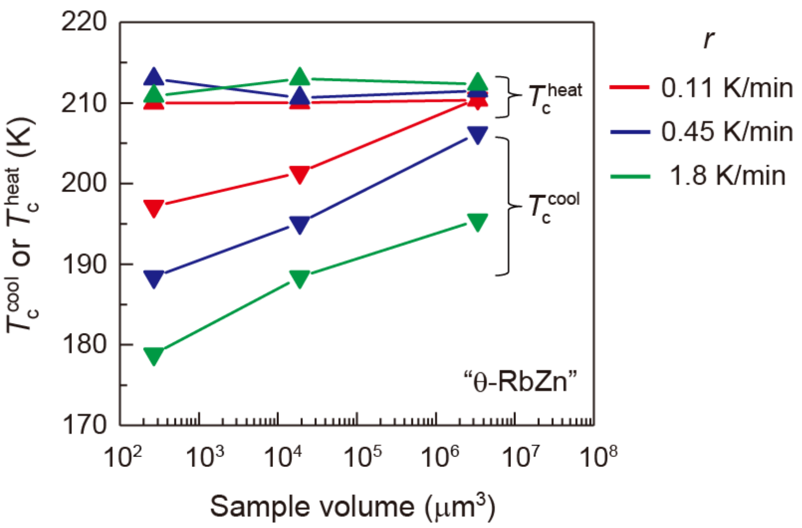


Fig. S12: $T_c^{cool}$ and $T_c^{heat}$ variations, defined by the transition-onset temperatures as shown in Fig. S11, for $\theta$-(BEDT-TTF)$_2$RbZn(SCN)$_4$.

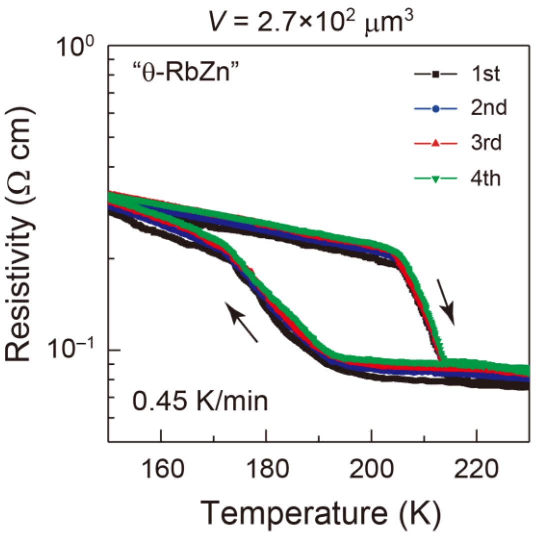


Fig. S13: Reproducibility of the temperature-resistivity profiles of θ-(BEDT-TTF)$_2$RbZn(SCN)$_4$ with $V = 2.7 \times 10^2$ μm$^3$. The thermal cycle was measured four times at a temperature sweep rate of 0.45 K/min.

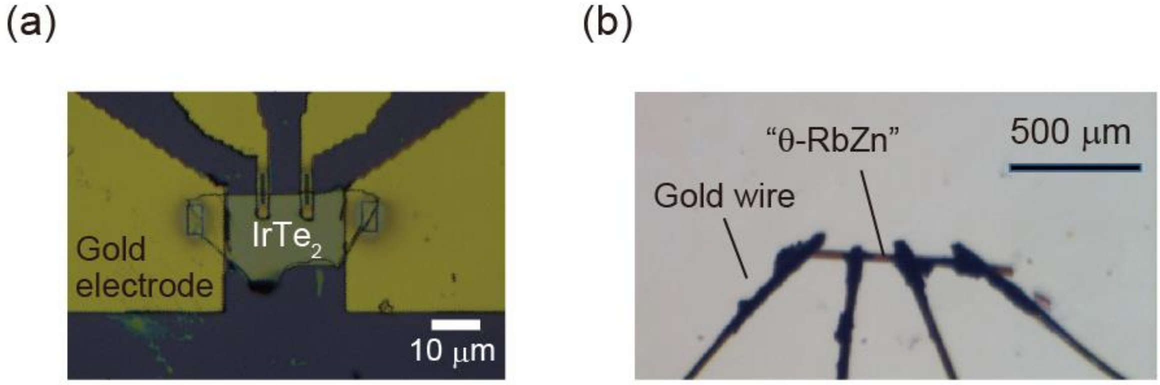


Fig. S14: Photograph of the sample configurations: (a) submicrometer-thick $IrTe_2$ and (b) θ-(BEDT-TTF)$_2$RbZn(SCN)$_4$ microcrystal.
